# Supplementary material for: A Bayesian hierarchical model for methane emission source apportionment
Source: arXiv:2506.03395 ancillary file (2026-03-24)
Supplement: Supplementary file 1 [file SI.pdf]

Supporting Information for:

# A Bayesian hierarchical model for methane emission source apportionment

William S. Daniels, Douglas W. Nychka, and Dorit M. Hammerling

Department of Applied Mathematics and Statistics, Colorado School of Mines, Golden, Colorado 80401, United States

## Contents

**S1 In situ sensor description** 2

**S2 Functional form of dispersion parameters** 2

**S3 Derivation of full conditional distributions for the MDLQ model** 4

S3.1 Prior probability of an emission: $p(\theta_i|\xi)$ . . . . . 4

S3.2 Error variance: $p(\sigma^2|\xi)$ . . . . . 5

S3.3 Prior belief about degrees of freedom: $\nu$ . . . . . 6

S3.4 Autocorrelation coefficient: r . . . . . 6

S3.5 Emission rate scale: $p(\tau_i^2|\xi)$ . . . . . 7

S3.6 Emission rates: $p(\beta_i|\xi)$ . . . . . 8

S3.7 Spike-slab indicator: $p(z_i|\xi)$ . . . . . 11

**S4 Sensitivity study of inversion window length** 16

**S5 Information filtered MDLQ output** 17

**S6 Average error in emission rate estimate as a function of sample size** 18

**S7 Confusion matrices for source- and site-level detections** 19

**S8 Autocorrelation simulation study** 21

**S9 MDLQ model variant with Laplace errors** 22

**S10Form of the correlation matrix: R** 24

**S11Methane concentration data example from all sensors** 25

## S1 In situ sensor description

The methane sensors in this study use Near-IR Tunable Diode Laser Absorption Spectroscopy (TDLAS) and have an accuracy of ±2% and a precision of ≤ 0.125 ppm with 60 s averaging, as reported by the manufacturer (R. Mistry, personal communication, January 17, 2024). The anemometers used in this study have an accuracy of ±2% ±0.3 m/s and a resolution of 0.01 m/s for wind speed and an accuracy of ±2 degrees and a resolution of 0.1 degrees for wind direction, as reported by the manufacturer [1].

## S2 Functional form of dispersion parameters

The Gaussian puff model (GPM) described in the main text relies on two dispersion parameters, $\sigma_z$ and $\sigma_y$, that control the vertical and horizontal widths, respectively, of the puffs as they travel downwind. As stated in the main text, we calculate $\sigma_z$ and $\sigma_y$ using the EPA parameterization of the Pasquill-Gifford-Turner dispersion scheme [2–4]. Under this parameterization, both $\sigma_y$ and $\sigma_z$ are functions of stability class and monotonically increase with total distance traveled. Below we provide the exact functional form of this parameterization.

$$\begin{aligned} \sigma_z &= ax^b \\ \sigma_y &= 465.11628x \tan\Theta \\ \Theta &= 0.017453293(c - d\ln x), \end{aligned}$$

where $x$ is the downwind distance in kilometers. Note that the units of $\sigma_z$ and $\sigma_y$ are meters. The values of $a$, $b$, $c$, and $d$ are a function of stability class and downwind distance, $x$. Stability class is a metric that summarizes the degree of turbulence in the atmosphere between the ground and the planetary boundary layer; it can take six different values: A, B, C, D, E, F, which are a function of surface wind speed, solar insolation, and cloudiness. Solar insolation and cloudiness data can be challenging to obtain in practice, and we therefore parameterize the stability class solely as a function of wind speed and time of day for use in the MDLQ model. The following lookup tables (adapted from [4]) are used in the MDLQ model to obtain values for the stability class and the $a$, $b$, $c$, and $d$ parameters.

Table 1: Lookup table for the atmospheric stability class.

| Wind speed (m/s) | Day | Night |
|---|---|---|
| <2 | A-B | E-F |
| 2-3 | B | E-F |
| 3-5 | B-C | D-E |
| 5-6 | C-D | D |
| >6 | D | D |

Table 2: Lookup table for the $c$ and $d$ parameters of the dispersion model parameterization.

| Stability Class | c | d |
|---|---|---|
| A | 24.1670 | 2.5334 |
| B | 18.3330 | 1.8096 |
| C | 12.5000 | 1.0857 |
| D | 8.3330 | 0.72382 |
| E | 6.2500 | 0.54287 |
| F | 4.1667 | 0.36191 |

Table 3: Lookup table for the *a* and *b* parameters of the dispersion model parameterization.

| **Stability Class** | **x (km)** | **a** | **b** |
|---|---|---|---|
| A | <0.10 | 122.800 | 0.94470 |
| | 0.10 - 0.15 | 158.080 | 1.05420 |
| | 0.15 - 0.20 | 170.220 | 1.09320 |
| | 0.20 - 0.25 | 179.520 | 1.12620 |
| | 0.25 - 0.30 | 217.410 | 1.26440 |
| | 0.30 - 0.40 | 258.890 | 1.40940 |
| | 0.40 - 0.50 | 346.750 | 1.72830 |
| | >0.50 | 453.850 | 2.11660 |
| B | <0.20 | 90.673 | 0.93198 |
| | 0.20 - 0.40 | 98.483 | 0.98332 |
| | >0.40 | 109.300 | 1.09710 |
| C | All | 61.141 | 0.91465 |
| D | <0.30 | 34.459 | 0.86974 |
| | 0.30 - 1.00 | 32.093 | 0.81066 |
| | 1.00 - 3.00 | 32.093 | 0.64403 |
| | 3.00 - 10.00 | 33.504 | 0.60486 |
| | 10.00 - 30.00 | 36.650 | 0.56589 |
| | >30.00 | 44.053 | 0.51179 |
| E | <0.10 | 24.260 | 0.83660 |
| | 0.10 - 0.30 | 23.331 | 0.81956 |
| | 0.30 - 1.00 | 21.628 | 0.75660 |
| | 1.00 - 2.00 | 21.628 | 0.63077 |
| | 2.00 - 4.00 | 22.534 | 0.57154 |
| | 4.00 - 10.00 | 24.703 | 0.50527 |
| | 10.00 - 20.00 | 26.970 | 0.46713 |
| | 20.00 - 40.00 | 35.420 | 0.37615 |
| | >40.00 | 47.618 | 0.29592 |
| F | <0.20 | 15.209 | 0.81558 |
| | 0.20 - 0.70 | 14.457 | 0.78407 |
| | 0.70 - 1.00 | 13.953 | 0.68465 |
| | 1.00 - 2.00 | 13.953 | 0.63227 |
| | 2.00 - 3.00 | 14.823 | 0.54503 |
| | 3.00 - 7.00 | 16.187 | 0.46490 |
| | 7.00 - 15.00 | 17.836 | 0.41507 |
| | 15.00 - 30.00 | 22.651 | 0.32681 |
| | 30.00 - 60.00 | 27.074 | 0.27436 |
| | >60.00 | 34.219 | 0.21716 |

## S3 Derivation of full conditional distributions for the MDLQ model

Many of the following derivations are based on [5]. In particular, we follow the methodology presented in [5] for integrating out $\beta_i$ from the conditional distribution for $z_i$.

### S3.1 Prior probability of an emission: $p(\theta_i|\xi)$

The full conditional for $\theta_i$ reduces to a relatively simple expression given the conditional independencies of the model hierarchy. We can write

$$\begin{aligned}
p(\theta_i|\xi) &= p(\theta_i|z_i) \\
&= \frac{p(\theta_i, z_i)}{p(z)} \\
&= \frac{p(z_i|\theta_i)p(\theta_i)}{p(z)} \\
&= \frac{p(z_i|\theta_i)p(\theta_i)}{\int p(z|\theta_i)p(\theta_i)d\theta_i} \\
&= \frac{1}{c}p(z_i|\theta_i)p(\theta_i),
\end{aligned}$$

where we have absorbed the normalizing integral into the constant $c$. Plugging in the prior distributions for $z_i$ and $\theta_i$ gives

$$\begin{aligned}
p(\theta_i|\xi) &= \frac{1}{c}\theta_i^{z_i}(1-\theta_i)^{1-z_i}\frac{1}{B(a_i, b_i)}\theta_i^{a_i-1}(1-\theta_i)^{b_i-1} \\
&= \frac{1}{c}\theta_i^{z_i+a_i-1}(1-\theta_i)^{1-z_i+b_i-1}.
\end{aligned}$$

This is the unnormalized probability density function of a Beta distribution, and therefore we can update $\theta_i$ by drawing from

$$\theta_i|\xi \sim \text{Beta}(z_i + a_i, 1 - z_i + b_i).$$

Note that the conditional posterior for $\theta_i$ depends only on $z_i$ and its fixed prior parameters. This means that we cannot gain much information about this parameter, as $z_i$ can only takes values 0 and 1. For example, if we use a uniform prior on $\theta_i$ (i.e., $a_i = 1$ and $b_i = 1$), then the conditional posterior can be only $\text{Beta}(1, 2)$ or $\text{Beta}(2, 1)$.

### S3.2 Error variance: $p(\sigma^2|\xi)$

Similar to $\theta_i$, the full conditional for $\sigma^2$ reduces to a relatively simple expression given the conditional independencies of the model. We can write

$$\begin{aligned}
p(\sigma^2|\xi) &= p(\sigma^2|y,\beta,r,\nu) \\
&= \frac{p(\sigma^2,y,\beta,r,\nu)}{p(y,\beta,r,\nu)} \\
&= \frac{p(y|\sigma^2,\beta,r,\nu)p(\sigma^2,\beta,r,\nu)}{p(y,\beta,r,\nu)} \\
&= \frac{p(y|\sigma^2,\beta,r,\nu)p(\sigma^2|\beta,r,\nu)p(\beta|r,\nu)p(r|\nu)p(\nu)}{p(y|\beta,r,\nu)p(\beta|r,\nu)p(r|\nu)p(\nu)} \\
&= \frac{p(y|\sigma^2,\beta,r,\nu)p(\sigma^2|\beta,r,\nu)}{p(y|\beta,r,\nu)} \\
&= \frac{p(y|\sigma^2,\beta,r,\nu)p(\sigma^2|\nu)}{p(y|\beta,r,\nu)} \\
&= \frac{p(y|\sigma^2,\beta,r,\nu)p(\sigma^2|\nu)}{\int p(y|\sigma^2,\beta,r,\nu)p(\sigma^2|\nu)d\sigma^2} \\
&= \frac{1}{c}p(y|\sigma^2,\beta,r,\nu)p(\sigma^2|\nu),
\end{aligned}$$

where we have again absorbed the normalizing integral into the constant $c$. We also absorb all terms that are not a function of $\sigma^2$ into the normalizing constant. Plugging in expressions for the likelihood and the $\sigma^2$ prior gives

$$\begin{aligned}
p(\sigma^2|\xi) &= \frac{1}{c}(\sigma^2 R)^{-1/2}\exp\left(\frac{1}{2\sigma^2}(y-X\beta)^T R^{-1}(y-X\beta)\right)(\sigma^2)^{-\nu/2-1}\exp\left(-\frac{\nu/2}{\sigma^2}\right) \\
&= \frac{1}{c}(\sigma^2)^{-n/2}(\sigma^2)^{-\nu/2-1}\exp\left(-\frac{1}{\sigma^2}\left(\frac{\nu}{2}+\frac{(y-X\beta)^T R^{-1}(y-X\beta)}{2}\right)\right) \\
&= \frac{1}{c}(\sigma^2)^{-(n/2+\nu/2)-1}\exp\left(-\frac{1}{\sigma^2}\left(\frac{\nu}{2}+\frac{(y-X\beta)^T R^{-1}(y-X\beta)}{2}\right)\right).
\end{aligned}$$

This is the unnormalized probability density function of an Inverse Gaussian distribution, and we can therefore update $\sigma^2$ by drawing from

$$\sigma^2|\xi \sim \text{Inv-Gamma}\left(\frac{\nu}{2}+\frac{n}{2}, \frac{\nu}{2}+\frac{1}{2}(y-X\beta)^T R^{-1}(y-X\beta)\right).$$

Unlike $\theta_i$, we update $\sigma^2$ using all $n$ data points contained in $y$ and all of the $p$ emission rate estimates. Therefore, we can glean notably more information about the error variance than the prior probability of an emission.

### S3.3 Prior belief about degrees of freedom: $\nu$

The prior for $\sigma^2$ was set such that in the prior model (i.e., before seeing the data), the $\epsilon$ would be distributed according to a Student's t-distribution with $\nu$ degrees of freedom. We begin with

$$\begin{aligned} p(\nu|\xi) &= p(\nu|\sigma^2) \\ &= \frac{p(\nu, \sigma^2)}{p(\sigma^2)} \\ &= \frac{p(\sigma^2|\nu)p(\nu)}{p(\sigma^2)} \\ &= \frac{p(\sigma^2|\nu)p(\nu)}{\int p(\sigma^2|\nu)p(\nu)d\nu} \\ &= \frac{1}{c}p(\sigma^2|\nu)p(\nu), \end{aligned}$$

Unfortunately, this conditional will not take a convenient form, and we must therefore sample from it using a Metropolis-Hastings step. We use the log of the following as the target distribution:

$$p(\nu|\xi) = \frac{1}{c}\frac{(\nu/2)^{\nu/2}}{\Gamma(\nu/2)}(\sigma^2)^{-(\nu/2)-1}\exp\left(\frac{-\nu/2}{\sigma^2}\right)\nu^{-\alpha_1-1}\exp\left(\frac{-\alpha_2}{\nu}\right).$$

### S3.4 Autocorrelation coefficient: r

The derivation of the conditional for $r$ is very similar to that for $\sigma^2$, as they are in similar positions within the model hierarchy. We begin with

$$\begin{aligned} p(r|\xi) &= p(r|y, \beta, \sigma^2) \\ &= \frac{p(r, y, \beta, \sigma^2)}{p(y, \beta, \sigma^2)} \\ &= \frac{p(y|\sigma^2, \beta, r)p(\sigma^2, \beta, r)}{p(y, \beta, \sigma^2)} \\ &= \frac{p(y|\sigma^2, \beta, r)p(r|\beta, \sigma^2)p(\beta|\sigma^2)p(\sigma^2)}{p(y|\beta, \sigma^2)p(\beta|\sigma^2)p(\sigma^2)} \\ &= \frac{p(y|\sigma^2, \beta, r)p(r|\beta, \sigma^2)}{p(y|\beta, \sigma^2)} \\ &= \frac{p(y|\sigma^2, \beta, r)p(r)}{\int p(y|\beta, \sigma^2, r)p(r)dr} \\ &= \frac{1}{c}p(y|\sigma^2, \beta, r)p(r), \end{aligned}$$

where we have again absorbed the normalizing integral into the constant $c$. Because the prior on $r$ is a uniform distribution, we end up with simply

$$r|\xi \sim \begin{cases} N(X\beta, \sigma^2 R) & 0 < r < 1 \\ 0 & \text{otherwise.} \end{cases}$$

### S3.5 Emission rate scale: $p(\tau_i^2|\xi)$

We again begin by using the structure of the hierarchy to simplify the full conditional. We can write

$$\begin{aligned} p(\tau_i^2|\xi) &= p(\tau_i^2|\beta_i, z_i) \\ &= \frac{p(\tau_i^2, \beta_i, z_i)}{p(\beta_i, z_i)} \\ &= \frac{p(\beta_i|\tau_i^2, z_i)p(\tau_i^2, z_i)}{p(\beta_i, z_i)} \\ &= \frac{p(\beta_i|\tau_i^2, z_i)p(\tau_i^2|z_i)p(z_i)}{p(\beta_i|z_i)p(z_i)} \\ &= \frac{p(\beta_i|\tau_i^2, z_i)p(\tau_i^2|z_i)}{p(\beta_i|z_i)} \\ &= \frac{p(\beta_i|\tau_i^2, z_i)p(\tau_i^2)}{p(\beta_i|z_i)} \\ &= \frac{p(\beta_i|\tau_i^2, z_i)p(\tau_i^2)}{\int p(\beta_i|\tau_i^2, z_i)p(\tau_i^2)d\tau_i^2} \\ &= \frac{1}{c}p(\beta_i|\tau_i^2, z_i)p(\tau_i^2), \end{aligned}$$

were we have absorbed the normalizing integral into the constant $c$. Unlike the previous parameters, the conditional posterior for $\tau_i^2$ depends on the $\beta_i$ prior, which is conditioned on $z_i$. To evaluate this expression, we will consider the cases where $z_i = 0$ and $z_i = 1$ separately. We begin with the $z_i = 1$ case, where we have that

$$\begin{aligned} p(\tau_i^2|\beta_i, z_i) &= \frac{1}{c}p(\beta_i|\tau_i^2, z_i = 1)p(\tau_i^2) \\ &= \frac{1}{c}\frac{1}{\tau_i^2\sigma^2}\exp\left(\frac{\beta_i}{\tau_i^2\sigma^2}\right)\frac{d_i^{c_i}}{\Gamma(c_i)}(\tau_i^2)^{-(c_i+1)}\exp\left(\frac{-d_i}{\tau_i^2}\right). \end{aligned}$$

Note that all terms that do not depend on the parameter of interest, $\tau_i^2$, will cancel with the terms that have been absorbed into the normalizing constant, $c$. For simplicity, we can absorb these terms into $c$, giving

$$\begin{aligned} p(\tau_i^2|\beta_i, z_i = 1) &= \frac{1}{c}(\tau_i^2)^{-1-c_i-1}\exp\left(\frac{-\beta_i}{\tau_i^2\sigma^2} - \frac{d_i}{\tau_i^2}\right) \\ &= \frac{1}{c}(\tau_i^2)^{-((1+c_i)+1)}\exp\left(-\left(\frac{\beta_i}{\sigma^2} + d_i\right)/\tau_i^2\right). \end{aligned}$$

This is the unnormalized probability density function of an Inverse Gamma distribution, and hence we can update $\tau_i^2$ for the $z_i = 1$ case by drawing from

$$\tau_i^2 | \beta_i, z_i = 1 \sim \text{Inv-Gamma}\left(1 + c_i, \frac{\beta_i}{\sigma^2} + d_i\right).$$

We now consider the case where $z_i = 0$. Recall that $\beta_i = 0$ when $z_i = 0$, and hence in this case we sample $\tau_i^2$ from its prior distribution:

$$\tau_i^2 | \beta_i, z_i = 0 \sim \text{Inv-Gamma}(c_i, d_i).$$

We again briefly consider the information content of this conditional posterior. We update $\tau_i^2$ using only information contained in the $i^{\text{th}}$ emission rate estimate (which may be equal to zero is $z_i = 0$). This utilizes slightly more information than the conditional posterior for $\theta_i$, which depends only on the discrete parameter $z_i$, but less than the conditional posterior for $\sigma^2$, which depends on the entire $\beta$ vector and the data $y$.

## S3.6 Emission rates: $p(\beta_i|\xi)$

Unlike the previous parameters, $\beta_i$ is conditionally dependent on many of the other parameters. Therefore, our first simplification step, while following the same logic as the other parameters, is slightly more complex. For notational clarity, let $\beta_{-i} = \{\beta_1, ..., \beta_{i-1}, \beta_{i+1}, ..., \beta_p\}$. We start by writing

$$p(\beta_i|\xi) = p(\beta_i|\beta_{-i}, y, \tau_i^2, z_i, \sigma^2, r),$$

and we again consider the $z_i = 0$ and $z_i = 1$ cases separately. By definition, $\beta_i = 0$ when $z_i = 0$. Now consider the case where $z_i = 1$. We have that

$$\begin{aligned}
p(\beta_i|\xi) &= p(\beta_i|y, \beta_{-i}, z_i = 1, \tau_i^2, \sigma^2, r) \\
&= \frac{p(y, \beta_i, \beta_{-i}, z_i = 1, \tau_i^2, \sigma^2, r)}{p(y, \beta_{-i}, z_i = 1, \tau_i^2, \sigma^2, r)} \\
&= \frac{p(y|\beta_i, \beta_{-i}, z_i = 1, \tau_i^2, \sigma^2, r)p(\beta_i|\beta_{-i}, z_i = 1, \tau_i^2, \sigma^2, r)p(\beta_{-i}, z_i = 1, \tau_i^2, \sigma^2, r)}{p(y|\beta_{-i}, z_i = 1, \tau_i^2, \sigma^2, r)p(\beta_{-i}, z_i = 1, \tau_i^2, \sigma^2, r)} \\
&= \frac{p(y|\beta_i, \beta_{-i}, z_i = 1, \tau_i^2, \sigma^2, r)p(\beta_i|\beta_{-i}, z_i = 1, \tau_i^2, \sigma^2, r)}{p(y|\beta_{-i}, z_i = 1, \tau_i^2, \sigma^2, r)}.
\end{aligned}$$

We can simplify the $\beta_i$ prior given the independence structure of the hierarchy. Note that $\beta_i \perp\!\!\!\perp \beta_{-i}$, $\beta_i \perp\!\!\!\perp \sigma^2$, and $\beta_i \perp\!\!\!\perp r$ given that we do not condition on $y$. Therefore, we get that

$$\begin{aligned}
p(\beta_i|\xi) &= \frac{p(y|\beta_i, \beta_{-i}, z_i = 1, \tau_i^2, \sigma^2, r)p(\beta_i|z_i = 1, \tau_i^2)}{p(y|\beta_{-i}, z_i = 1, \tau_i^2, \sigma^2, r)} \\
&= \frac{p(y|\beta_i, \beta_{-i}, z_i = 1, \tau_i^2, \sigma^2, r)p(\beta_i|z_i = 1, \tau_i^2)}{\int p(y|\beta_i, \beta_{-i}, z_i = 1, \tau_i^2, \sigma^2, r)p(\beta_i|z_i = 1, \tau_i^2)d\beta_i} \\
&= \frac{1}{c}p(y|\beta_i, \beta_{-i}, z_i = 1, \tau_i^2, \sigma^2, r)p(\beta_i|z_i = 1, \tau_i^2),
\end{aligned}$$

where we have again absorbed the normalizing integral into the constant $c$. Plugging in expressions for the likelihood and the $\beta_i$ prior gives

$$\begin{aligned}
p(\beta_i|\xi) &= \frac{1}{c}\exp\left(-\frac{1}{2\sigma^2}(y - X\beta)^T R^{-1}(y - X\beta)\right)\exp\left(-\frac{\beta_i}{\tau_i^2\sigma^2}\right) \qquad (1)\\
&= \frac{1}{c}\exp\left(-\frac{1}{2\sigma^2}(y^T R^{-1} y - 2y^T R^{-1} X\beta + \beta^T X^T R^{-1} X\beta) - \frac{\beta_i}{\tau_i^2\sigma^2}\right)\\
&= \frac{1}{c}\exp\left(-\frac{1}{2}\left(\frac{-2y^T R^{-1} X\beta}{\sigma^2} + \frac{\beta^T X^T R^{-1} X\beta}{\sigma^2} + \frac{2\beta_i}{\tau_i^2\sigma^2}\right)\right)\\
&= \frac{1}{c}\exp\left(-\frac{1}{2}\left(\beta^T\left(\frac{X^T R^{-1} X}{\sigma^2}\right)\beta - \frac{2y^T R^{-1} X\beta}{\sigma^2} + \frac{2e_i^T\beta}{\tau_i^2\sigma^2}\right)\right),
\end{aligned}$$

where $e_i = \{0, ..., 0, 1, 0, ..., 0\} \in \mathbb{R}^{1xp}$ is a vector of zeros with a one in the $i^{\text{th}}$ entry. Further simplifying gives

$$\begin{aligned}
p(\beta_i|\xi) &= \frac{1}{c}\exp\left(-\frac{1}{2}\left(\beta^T\left(\frac{X^T R^{-1} X}{\sigma^2}\right)\beta - 2\left(\frac{y^T R^{-1} X}{\sigma^2} - \frac{e_i^T}{\tau_i^2\sigma^2}\right)\beta\right)\right)\\
&= \frac{1}{c}\exp\left(-\frac{1}{2}\left(\beta^T\left(\frac{X^T R^{-1} X}{\sigma^2}\right)\beta - 2\left(\frac{X^T R^{-1} y}{\sigma^2} - \frac{e_i}{\tau_i^2\sigma^2}\right)^T\beta\right)\right).
\end{aligned}$$

We can now complete the square to convert this expression to a more familiar form. Let

$$\begin{aligned}
\mu &= \left(\frac{X^T R^{-1} X}{\sigma^2}\right)^{-1}\left(\frac{X^T R^{-1} y}{\sigma^2} - \frac{e_i}{\tau_i^2\sigma^2}\right)\\
\Sigma &= \left(\frac{X^T R^{-1} X}{\sigma^2}\right)^{-1}\\
g &= \left(\frac{X^T R^{-1} y}{\sigma^2} - \frac{e_i}{\tau_i^2\sigma^2}\right)^T\left(\frac{X^T R^{-1} X}{\sigma^2}\right)^{-1}\left(\frac{X^T R^{-1} y}{\sigma^2} - \frac{e_i}{\tau_i^2\sigma^2}\right).
\end{aligned}$$

Plugging in these expressions gives

$$\begin{aligned}
p(\beta_i|\xi) &= \frac{1}{c}\exp\left(-\frac{1}{2}((\beta - \mu)^T\Sigma(\beta - \mu) - g)\right)\\
&= \frac{1}{c}\exp\left(-\frac{1}{2}(\beta - \mu)^T\Sigma(\beta - \mu)\right)\exp(-g),
\end{aligned}$$

and since the $\exp(-g)$ term does not depend on $\beta_i$, we can absorb it into the scaling constant, $c$. We now have that

$$p(\beta_i|\xi) = \frac{1}{c}\exp\left(-\frac{1}{2}(\beta - \mu)^T\Sigma(\beta - \mu)\right),$$

which is of course an unscaled, multivariate Normal distribution. Therefore, we can update $\beta_i$ by sampling from

$$\beta_i|\xi \sim \begin{cases} 0 & z_i = 0 \\ \mathcal{N}\left( (\frac{X^T R^{-1} X}{\sigma^2})^{-1} (\frac{X^T R^{-1} y}{\sigma^2} - \frac{e_i}{\tau_i^2 \sigma^2}), (\frac{X^T R^{-1} X}{\sigma^2})^{-1} \right) & z_i = 1. \end{cases}$$

We pause here to raise an important point about the support of $\beta_i$. The prior on $\beta_i$ follows an exponential distribution when $z_i = 1$, which has non-negative support. Therefore, we also limit the support of $\beta_i$ to $[0, \infty]$ kg/hr when we introduce the exponential prior in Equation 1. This is a desired feature of the MDLQ model, as methane sinks (i.e., negative emission rates) are unlikely on oil and gas sites. However, sampling from a truncated normal above 0 kg/hr can be challenging when a vast majority of the distribution's mass is below 0 kg/hr. Our procedure for sampling the $\beta_i$ update in this scenario is described below.

We first try an inverse transform to sample the tail of the $\beta_i$ update. For simplicity, we break this process up into two steps. We first use the inverse transform to sample from a standard normal, which we then transform into a sample from the multivariate normal that is the $\beta_i|\xi$ update using the Cholesky decomposition of $\Sigma$,

$$\Sigma = LL^{\mathrm{T}},$$

where $L$ is a lower triangular matrix with real and positive entries. Therefore, a sample from the $\beta_i$ update can be computed as

$$x = \mu + L\Phi^{-1}(U),$$

where $U \sim$ Uniform(0,1) and the update for $\beta_i$ is just $x_i$. To make sampling from the tail more efficient, we iteratively limit the support of $U$ to higher percentiles until a sample, $x_i$, above 0 kg/hr is obtained. This procedure provides exact samples from the $\beta_i$ update. However, if we attempt to limit the support of $U$ beyond approximately $[1 - 10^{-14}, 1]$, then numerical precision issues arise as the support of $U$ is rounded to $[1, 1]$, making it impossible to generate samples. This occurs when 0 kg/hr is about 6 standard deviations above $\mu_i$.

When the inverse transform is no longer able to provide an exact sample from the tail of the $\beta_i$ update, we transition to an approximation based on the Mills Ratio. The Mills Ratio for a continuous random variable $Z$ is given by

$$m(z) \equiv \frac{\bar{F}(z)}{f(z)},$$

where $\bar{F}(z) = P(Z > z)$ is the complementary CDF and $f(z)$ is the pdf. If $Z$ is a standard normal, then

$$m(z) \approx \frac{1}{z}$$

as $x \longrightarrow \infty$ [6]. Therefore, we have that

$$\bar{F} \approx \frac{f(z)}{z}.$$

Now we will use the Mills Ratio to approximate a sample from the standard normal above a given threshold, $b$. We start with a sample $U \sim$ Uniform(0,1), which we then transform to a sample from the tail of a standard normal above threshold $b$. To derive this transformation, we first set $U$ equal to the desired conditional probability:

$$\begin{aligned} U \sim \text{Uniform(0,1)} &= P(Z > z | Z > b) \\ &= \frac{P(Z > z) \cap P(Z > b)}{P(Z > b)} = \frac{P(Z > z)}{P(Z > b)}, \end{aligned}$$

where the last equality comes from the fact that we are interested in the situation where $z \geq b$, which implies that $\{Z > z\} \subset \{Z > b\}$. We can then apply the Mills Ratio approximation to get

$$\begin{aligned} U &= \frac{P(Z > z)}{P(Z > b)} \\ &= \frac{\bar{F}(z)}{\bar{F}(b)} \\ &\approx \frac{f(z)/z}{f(b)/b} \\ &\approx \frac{b}{z}\exp\{-(z^2 - b^2)/2\}. \end{aligned}$$

Next we take the log of both sides to linearize the equation, dropping the $\log(z)$ term as this becomes insignificant for large $z$. Solving for $z$ as a function of $U$ gives

$$\begin{aligned} \log(U) &\approx \log(b) - \log(z) - \frac{z^2 - b^2}{2} \\ \log(U) &\approx \log(b) - \frac{z^2 - b^2}{2} \\ 2\log(U) &\approx 2\log(b) - z^2 + b^2 \\ z^2 &\approx b^2 - 2(\log(U) - \log(b)) \\ z^2 &\approx b^2 - 2\log(U/b) \\ z &\approx \sqrt{b^2 - 2\log(U/b)}. \end{aligned} \tag{2}$$

Equation 2 now provides an approximate transformation of a uniform sample into a sample from the standard normal conditioned on $z \geq b$. Finally, we again use the Cholesky decomposition to transform $z$ into a sample from the multivariate normal that is the $\beta_i|\xi$ update:

$$x = \mu + Lz,$$

where the update for $\beta_i$ is again just $x_i$. To generate a tail sample in extreme situations, we simply increase $b$ iteratively until a sample, $x_i$, above 0 kg/hr is obtained.

### S3.7 Spike-slab indicator: $p(z_i|\xi)$

Since $z_i$ takes discrete values $\{0, 1\}$, its conditional posterior distribution can be written as

$$z_i|\xi \sim \text{Bernoulli}(\psi_i),$$

where

$$\psi_i = \frac{p(z_i = 1|\xi)}{p(z_i = 0|\xi) + p(z_i = 1|\xi)}.$$

We now examine the $p(z_i|\xi)$ term. Given the structure of the hierarchy, we can write

$$p(z_i|\xi) = p(z_i|\beta_i, \tau_i^2, \theta_i).$$

However, this conditional poses a new challenge given the presence of the Dirac delta function in the prior on $\beta_i$. Specifically, if we were to expand this conditional in a similar fashion to the other parameters, then the $\psi_i$ ratio would have a Dirac delta function in the denominator. This means that $z_i$ draws of 0 would result in $\beta_i$ draws of 0 (by definition), which would in turn result in a $\psi_i$ ratio of 0. This means that the subsequent $z_i$ draw would also be 0, and this cycle would repeat. In other words, the presence of the Dirac delta function would make it impossible for the Gibbs sampler to leave the $\beta_i = 0$ regime, and hence the Markov chain would not achieve proper mixing.

To avoid this issue, we will integrate $\beta_i$ out of the conditional distribution, which bypasses the intractable Dirac delta function. We start by conditioning $z_i$ on all parameters, despite some of them being conditionally independent. This will make it easier to integrate out $\beta_i$ in the following steps. Also note that, for brevity, we skip directly to absorbing the normalizing constant into the $c$ term. We have that

$$\begin{aligned} p(z_i|\xi) &= p(z_i|y, z_{-i}, \beta_{-i}, \beta_i, \sigma^2, \tau^2, \theta, r) \\ &= \frac{1}{c} p(y|z, \beta_{-i}, \beta_i, \sigma^2, \tau^2, \theta, r) p(\beta_i|z, \beta_{-i}, \sigma^2, \tau^2, \theta, r) p(\beta_{-i}|z, \sigma^2, \tau^2, \theta, r) p(z|\sigma^2, \tau^2, \theta, r) p(\sigma^2) p(\tau^2) p(\theta) p(r). \end{aligned}$$

We can simplify this expression by unconditioning on parameters that are conditionally independent, giving

$$p(z_i|\xi) = \frac{1}{c} p(y|\beta_{-i}, \beta_i, \sigma^2, r) p(\beta_i|z_i, \tau_i^2) p(\beta_{-i}|z_{-i}, \tau_{-i}^2) p(z|\theta) p(\sigma^2) p(\tau^2) p(\theta) p(r).$$

Terms that appear in both the $z_i = 0$ and $z_i = 1$ cases will cancel out in the $\psi_i$ ratio, and hence we can absorb them into the $c$ term at this point for brevity. This gives

$$p(z_i|\xi) = \frac{1}{c} p(y|\beta_{-i}, \beta_i, \sigma^2, r) p(\beta_i|z_i, \tau_i^2) p(z|\theta).$$

We can now integrate out $\beta_i$:

$$p(z_i|\xi) = \frac{1}{c} p(z|\theta) \int p(y|\beta_{-i}, \beta_i, \sigma^2, r) p(\beta_i|z_i, \tau_i^2) d\beta_i.$$

To evaluate this integral, we again consider the $z_i = 0$ and $z_i = 1$ cases separately. We begin with $z_i = 0$. Recall that in this case, $\beta_i = 0$. Before proceeding, we first introduce some new notation. Let $X_{i,\bullet}$ denote the $i^{\text{th}}$ row of $X$ and $X_{\bullet,i}$ denote the $i^{\text{th}}$ column of $X$. Similarly, let $X_{-i,\bullet}$ denote $X$ with the $i^{\text{th}}$ row removed and $X_{\bullet,i}$ denote $X$ with the $i^{\text{th}}$ column removed. Now, the expression becomes

$$\begin{aligned} p(z_i = 0|\xi) &= \frac{1}{c} p(z|\theta) \det(\sigma^2 R)^{-1/2} \int \exp\left(-\frac{1}{2\sigma^2}(y - X\beta)^T R^{-1}(y - X\beta)\right) \delta_0(\beta_i) d\beta_i \\ &= \frac{1}{c} p(z|\theta) \det(\sigma^2 R)^{-1/2} \exp\left(-\frac{1}{2\sigma^2}(y - X_{\bullet,-i}\beta_{-i})^T R^{-1}(y - X_{\bullet,-i}\beta_{-i})\right) \int \delta_0(\beta_i) d\beta_i \\ &= \frac{1}{c} p(z|\theta) \det(\sigma^2 R)^{-1/2} \exp\left(-\frac{1}{2\sigma^2}(y - X_{\bullet,-i}\beta_{-i})^T R^{-1}(y - X_{\bullet,-i}\beta_{-i})\right), \end{aligned}$$

since $X\beta = X_{\bullet,-i}\beta_{-i}$ when $\beta_i = 0$ and $\int \delta_0(\beta_i) d\beta_i = 1$ by definition. Note that all $z_i$'s are conditionally independent given the $\theta$ vector. Therefore,

$$\begin{aligned}
p(z|\theta) &= p(z_1|\theta)...p(z_p|\theta) \\
&= p(z_1|\theta_1)...p(z_p|\theta_p) \\
&= \sum_{j=1}^{p} \theta_j^{z_j}(1-\theta_j)^{1-z_j},
\end{aligned}$$

and we can write

$$p(z_i = 0|\xi) = \frac{1}{c}\sum_{j=1}^{p} \theta_j^{z_j}(1-\theta_j)^{1-z_j} \det(\sigma^2 R)^{-1/2} \exp\left(-\frac{1}{2\sigma^2}(y - X_{\bullet,-i}\beta_{-i})^T R^{-1}(y - X_{\bullet,-i}\beta_{-i})\right).$$

However, note that all values $j \neq i$ of the sum will be the same in both the $z_i = 0$ and $z_i = 1$ cases. As before, these terms will cancel in the $\psi_i$ ratio and hence can be absorbed into the $c$ constant at this point. This leaves us with

$$p(z_i = 0|\xi) = \frac{1}{c}(1-\theta_i) \det(\sigma^2 R)^{-1/2} \exp\left(-\frac{1}{2\sigma^2}(y - X_{\bullet,-i}\beta_{-i})^T R^{-1}(y - X_{\bullet,-i}\beta_{-i})\right).$$

Now we consider the $z_i = 1$ case. The integral becomes

$$p(z_i = 1|\xi) = \frac{1}{c}p(z|\theta)\int \det(\sigma^2 R)^{-1/2} \exp\left(-\frac{1}{2\sigma^2}(y - X\beta)^T R^{-1}(y - X\beta)\right)\left(\frac{1}{\tau_i^2\sigma^2}\right)\exp\left(-\frac{\beta_i}{\tau_i^2\sigma^2}\right)d\beta_i.$$

Again, note that all $z_i's$ are conditionally independent, giving

$$p(z|\theta) = \sum_{j=1}^{p} \theta_j^{z_j}(1-\theta_j)^{1-z_j}.$$

Similar to the $z_i = 0$ case, all $j \neq i$ of the sum will be the same in both the $z_i = 0$ and $z_i = 1$ cases and hence will cancel. Therefore, we can absorb these terms into the $c$ constant. This leaves us with

$$p(z_i = 1|\xi) = \frac{1}{c}\theta_i \det(\sigma^2 R)^{-1/2}\left(\frac{1}{\tau_i^2\sigma^2}\right)\int \exp\left(-\frac{1}{2\sigma^2}(y - X\beta)^T R^{-1}(y - X\beta)\right)\exp\left(-\frac{\beta_i}{\tau_i^2\sigma^2}\right)d\beta_i.$$

For brevity, we will call the integral $A$, which we evaluate as follows:

$$\begin{aligned}
A &= \int \exp\left(-\frac{1}{2\sigma^2}(y - X\beta)^T R^{-1}(y - X\beta)\right)\exp\left(-\frac{\beta_i}{\tau_i^2\sigma^2}\right)d\beta_i \\
&= \int \exp\left(-\frac{1}{2\sigma^2}(y - X\beta)^T R^{-1}(y - X\beta) - \frac{\beta_i}{\tau_i^2\sigma^2}\right)d\beta_i.
\end{aligned}$$

We must now separate $\beta_i$ from the full $\beta$ vector. To do so, we first define some new terms. Let $y^* = R^{-1}y$ and $X^* = R^{-1}X$. Additionally, let $w = y - X_{\bullet,-i}\beta_{-i}$ and $w^* = R^{-1}y - R^{-1}X_{\bullet,-i}\beta_{-i}$. By linearity, we can write

$$
\begin{aligned}
(y - X\beta)^T R^{-1}(y - X\beta) &= \sum_{j=1}^{n}(y_j - X_{j,\bullet}\beta)(y_j^* - X_{j,\bullet}^*\beta) \\
&= \sum_{j=1}^{n}(y_j - X_{j,-i}\beta_{-i} + X_{j,i}\beta_i)(y_j^* - X_{j,-1}^*\beta_{-i} + X_{j,i}^*\beta_i) \\
&= \sum_{j=1}^{n}(w_j - X_{j,i}\beta_i)(w_j^* - X_{j,i}^*\beta_i).
\end{aligned}
$$

This formulation allows us to write the A integral as

$$
\begin{aligned}
A &= \int \exp\left(-\frac{1}{2\sigma^2}\sum_{j=1}^{n}(w_j - X_{j,i}\beta_i)(w_j^* - X_{j,i}^*\beta_i) - \frac{\beta_i}{\tau_i^2\sigma^2}\right)d\beta_i \\
&= \int \exp\left(-\frac{1}{2\sigma^2}\left(\sum w_j w_j^* - \sum w_j X_{j,i}^*\beta_i - \sum w_j^* X_{j,i}\beta_i + \sum X_{j,i}\beta_i X_{j,i}^*\beta_i\right) - \frac{\beta_i}{\tau_i^2\sigma^2}\right)d\beta_i \\
&= \exp\left(\frac{1}{2\sigma^2}\sum w_j w_j^*\right)\int \exp\left(-\frac{1}{2\sigma^2}\left(-\beta_i\sum(w_j X_{j,i}^* + w_j^* X_{j,i}) + \beta_i^2\sum X_{j,i}X_{j,i}^*\right) - \frac{\beta_i}{\tau_i^2\sigma^2}\right)d\beta_i.
\end{aligned}
$$

Again for brevity, we call the remaining integral $B$, which we evaluate as follows:

$$
\begin{aligned}
B &= \int \exp\left(-\frac{1}{2\sigma^2}\left(-\beta_i\sum(w_j X_{j,i}^* + w_j^* X_{j,i}) + \beta_i^2\sum X_{j,i}X_{j,i}^*\right) - \frac{\beta_i}{\tau_i^2\sigma^2}\right)d\beta_i \\
&= \int \exp\left(-\frac{1}{2\sigma^2}\left(-\beta_i\sum(w_j X_{j,i}^* + w_j^* X_{j,i}) + \beta_i^2\sum X_{j,i}X_{j,i}^* + \frac{2\beta_i}{\tau_i^2}\right)\right)d\beta_i \\
&= \int \exp\left(-\frac{1}{2\sigma^2}\left(\beta_i^2\sum X_{j,i}X_{j,i}^* - \beta_i\left(\sum(w_j X_{j,i}^* + w_j^* X_{j,i}) - \frac{2}{\tau_i^2}\right)\right)\right)d\beta_i \\
&= \int \exp\left(-\frac{\sum X_{j,i}X_{j,i}^*}{2\sigma^2}\left(\beta_i^2 - \beta_i\frac{\sum(w_j X_{j,i}^* + w_j^* X_{j,i}) - \frac{2}{\tau_i^2}}{\sum X_{j,i}X_{j,i}^*}\right)\right)d\beta_i \\
&= \int \exp\left(-\frac{\sum X_{j,i}X_{j,i}^*}{2\sigma^2}\left(\left(\beta_i - \frac{\sum(w_j X_{j,i}^* + w_j^* X_{j,i}) - \frac{2}{\tau_i^2}}{2\sum X_{j,i}X_{j,i}^*}\right)^2 - \left(\frac{\sum(w_j X_{j,i}^* + w_j^* X_{j,i}) - \frac{2}{\tau_i^2}}{2\sum X_{j,i}X_{j,i}^*}\right)^2\right)\right)d\beta_i \\
&= \exp\left(\frac{\left(\sum(w_j X_{j,i}^* + w_j^* X_{j,i}) - \frac{2}{\tau_i^2}\right)^2}{4\sigma^2\sum X_{j,i}X_{j,i}^*}\right)\int \exp\left(-\frac{\sum X_{j,i}X_{j,i}^*}{2\sigma^2}\left(\beta_i - \frac{\sum(w_j X_{j,i}^* + w_j^* X_{j,i}) - \frac{2}{\tau_i^2}}{2\sum X_{j,i}X_{j,i}^*}\right)^2\right)d\beta_i \\
&= \exp\left(\frac{\left(\sum(w_j X_{j,i}^* + w_j^* X_{j,i}) - \frac{2}{\tau_i^2}\right)^2}{4\sigma^2\sum X_{j,i}X_{j,i}^*}\right)\left(\frac{2\sigma^2\pi}{\sum X_{j,i}X_{j,i}^*}\right)^{1/2}\left(\frac{1}{2}\right),
\end{aligned}
$$

where we have used the following identity to evaluate the integral:

$$\int_{-\infty}^{\infty} \exp\left(-a(x+b)^2\right) dx = \left(\frac{\pi}{a}\right)^{1/2}.$$

Also note that an extra $(1/2)$ is introduced because the exponential prior on $\beta_i$ is zero for $\beta_i < 0$, and hence we only integrate over $[0, \infty]$. Recombining the $A$ and $B$ integrals gives us

$$p(z_i = 1|\xi) = \frac{1}{c}\theta_i \det(\sigma^2 R)^{-1/2} \left(\frac{1}{\tau_i^2\sigma^2}\right) \exp\left(\frac{1}{2\sigma^2}\sum w_j w_j^*\right)$$
$$\exp\left(\frac{\left(\sum(w_j X_{j,i}^* + w_j^* X_{j,i}) - \frac{2}{\tau_i^2}\right)^2}{4\sigma^2 \sum X_{j,i}X_{j,i}^*}\right)\left(\frac{2\sigma^2\pi}{\sum X_{j,i}X_{j,i}^*}\right)^{1/2}\left(\frac{1}{2}\right).$$

Finally, we can now construct an expression for the Bernoulli probability with which we will sample $z_i$. We have that

$$\begin{aligned}
\psi_i &= \frac{p(z_i = 1|\xi)}{p(z_i = 0|\xi) + p(z_i = 1|\xi)} \\
&= 1 - \frac{p(z_i = 0|\xi)}{p(z_i = 0|\xi) + p(z_i = 1|\xi)} \\
&= 1 - \frac{1-\theta_i}{(1-\theta_i) + \theta_i\left(\frac{1}{\tau_i^2\sigma^2}\right)\exp\left(\frac{\left(\sum_{j=1}^n (w_j X_{j,i}^* + w_j^* X_{j,i}) - \frac{2}{\tau_i^2}\right)^2}{4\sigma^2\sum_{j=1}^n X_{j,i}X_{j,i}^*}\right)\left(\frac{2\sigma^2\pi}{\sum_{j=1}^n X_{j,i}X_{j,i}^*}\right)^{1/2}\left(\frac{1}{2}\right)},
\end{aligned}$$

where again we draw $z_i$ from

$$z_i|\xi \sim \text{Bernoulli}(\psi_i).$$

## S4 Sensitivity study of inversion window length

We perform a sensitivity study of the length of the inversion window used in the main text, with results shown in Table 4. Specifically, we vary the length of the inversion window from 10 minutes to 60 minutes and run the MDLQ model on the METEC experiment for each length. We list a number of summary metrics in Table 4. The site-level inventory has a small dependence on inversion length, with a tendency to overestimate with short windows and a tendency to underestimate with long windows. The dependence of each source-level inventory to the inversion length varies by source. IQR increases slightly and coverage decreases as the length of the inversion window increases, except for the 60-minute window, which reverses this trend. Finally, the localization (i.e., alerting) accuracy decreases slightly as inversion length increases, again with the 60-minute window reversing the trend.

Table 4: Sensitivity study of inversion window length using data from the METEC experiment. Site-level total error is the error (estimate - truth) in the site-level inventory. The following five rows provide the source-level inventory errors (estimate - truth). Average site-level quantification error is the average error (estimate - truth) across all individual site-level emission rate estimates, and the IQR of these errors is the difference between their 25th and 75th percentiles. Coverage of the site-level 95% credible intervals is the fraction of inversion windows where the true site-level emission rate was contained within the 95% credible interval of the estimate. The average number of correct localization estimates is the average number of correct state estimates (either on or off) across all inversion windows.

| | **MDLQ 10min** | **MDLQ 20min** | **MDLQ 30min** | **MDLQ 40min** | **MDLQ 50min** | **MDLQ 60min** |
|---|---|---|---|---|---|---|
| **Site-level total error** | 1.4 t (20.3%) | 0.4 t (5.5%) | -0.1 t (-1.0%) | -0.3 t (-4.3%) | -0.5 t (-6.9%) | -0.4 t (-5.4%) |
| **West wellhead total error** | 0.3 t (17.9%) | 0.05 t (2.8%) | -0.1 t (-3.7%) | -0.1 t (-7.7%) | -0.1 t (-8.4%) | -0.04 t (-2.4%) |
| **West separator total error** | 0.1 t (5.5%) | -0.2 t (-17.9%) | -0.3 t (-22.0%) | -0.3 t (-26.5%) | -0.4 t (-29.5%) | -0.3 t (-26.1%) |
| **Tank total error** | 1.4 t (83.8%) | 1.3 t (73.7%) | 1.0 t (61.4%) | 1.0 t (58.3%) | 0.9 t (53.0%) | 0.8 t (45.4%) |
| **East wellhead total error** | -0.03 t (-2.8%) | -0.3 t (-22.3%) | -0.3 t (-26.3%) | -0.3 t (-28.3%) | -0.3 t (-30.5%) | -0.3 t (-25.2%) |
| **East separator total error** | -0.3 t (-27.4%) | -0.5 t (-35.5%) | -0.5 t (-38.8%) | -0.5 t (-41.5%) | -0.5 t (-42.8%) | -0.5 t (-40.7%) |
| **Avg site-level quant error** | 0.3 kg/hr | 0.07 kg/hr | -0.01 kg/hr | -0.05 kg/hr | -0.08 kg/hr | 0.06 kg/hr |
| **IQR of site-level quant errors** | 0.59 kg/hr | 0.69 kg/hr | 0.76 kg/hr | 0.82 kg/hr | 0.86 kg/hr | 0.52 kg/hr |
| **Site-level coverage of 95% CI** | 0.72 | 0.65 | 0.58 | 0.51 | 0.45 | 0.56 |
| **Avg number of correct localization estimates** | 4.00 out of 5 | 3.98 out of 5 | 3.79 out of 5 | 3.95 out of 5 | 3.94 out of 5 | 4.38 out of 5 |

# S5 Information filtered MDLQ output

In Section 4.1 of the main text, we postulate that errors in the source-level emissions inventories could be a result of inversion windows where the CMS data has information for a given source for only a subset of the window. Here we investigate this theory in more detail. Based on the location of the emission sources and the CMS sensors on the METEC site (see Figure 1 in the main text), there can be times when emitting methane is blown between adjacent sensors. When periods of no information like this happens, there will be no enhancements in the observed methane concentrations making it naively appear as if no emissions are occurring. When a period of no information for a given source spans an entire inversion window, we do not infer emission characteristics for that source. However, periods of information may only span a subset of the 30-minute inversion window. This is less likely to happen for the Tanks, as they are located in the center of the site and are further from the CMS sensors. Because of this geometry, methane plumes from the Tanks have more time to disperse (i.e., get wider) before reaching the sensors, making the CMS data more likely to contain information about this source. As a result, the MDLQ model may be incorrectly attributing emissions from the other four sources to the Tanks.

To test this, we identify all of the 30-minute inversion windows that have at least one sensor downwind of all potential sources for the entire window. We do so using the $X$ matrix as described in Section 3.4 in the main text. We then analyze the performance of the MDLQ model on only these inversion windows, with results shown in Figure S1. After filtering out the inversion windows that have partial information, the site-level inventory remains accurate with an error of only 1.7%. Additionally, the Tank inventory (which was previous overestimated) and the East Separator inventory (which was previous underestimated) are much closer to the truth with errors of -12.7% and -23.4%, respectively. This reduction in source-level inventory errors provides evidence that inversion windows with partial information are at least partially responsible for inaccuracies in the source-level inventories.

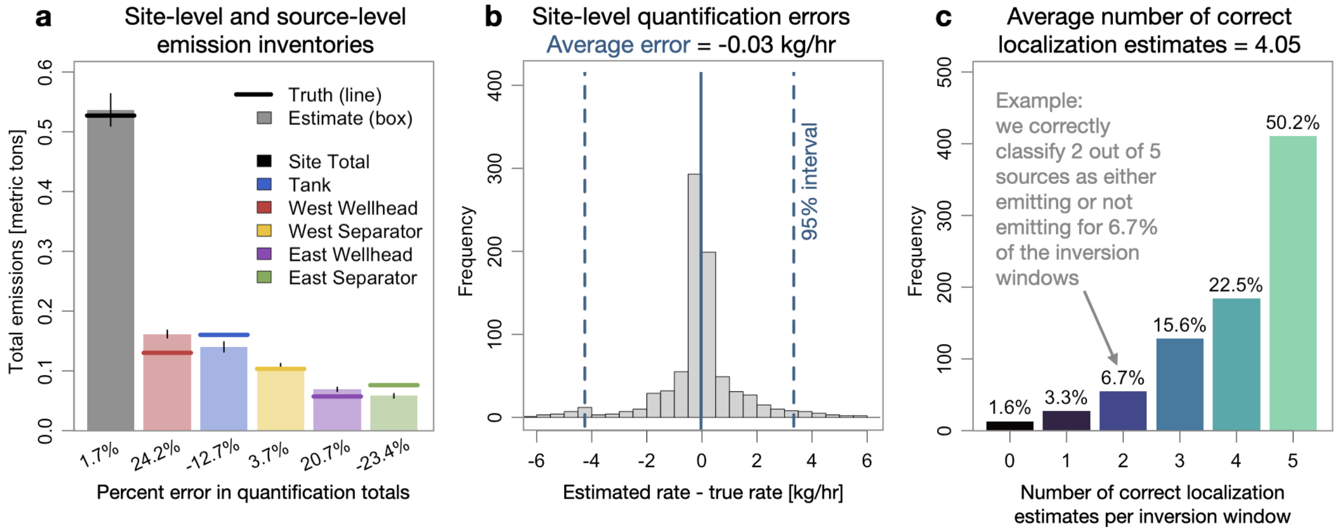


Figure S1: Summary of the source apportionment results for the METEC experiment after keeping only the 30-minute inversion windows that have at least one sensor downwind of all sources for the entire window. (a) Site- and source-level inventories created by summing the emission rate estimates across all inversion windows. Vertical lines show 95% confidence intervals. (b) Distribution of errors in the site-level emission rate estimates. (c) Alerting accuracy, where a correct localization estimate is a correct estimate of emission state (i.e., either emitting or not emitting).

## S6 Average error in emission rate estimate as a function of sample size

In Section 4.1 of the main text, we note that there is fairly high variability in the individual site-level emission rate estimates from the MDLQ model, but they are largely unbiased with an average error of -0.01 kg/hr. This raises the question: how many estimates do you need before their average is close to the true value? Here we answer this question by resampling all of the site-level emission rate estimates from the METEC experiment.

Specifically, we sample 5,000 times from all 30-minute inversion windows at different sample sizes ranging from 1 to 600. For each sample, we compute the average error between the estimated and true site-level emission rate. Figure S2 shows the distribution of these errors as a function of the number of site-level estimates included in the average. The black line shows the average of the average errors, the purple region shows the inner 95% of the average errors, and the green vertical line shows the point where the inner 95% is bounded by [-1, 1] kg/hr. Because the site-level estimates are largely unbiased, it takes only 21 estimates for the average error to be bounded by [-1, 1] kg/hr, corresponding to approximately 11 hours.

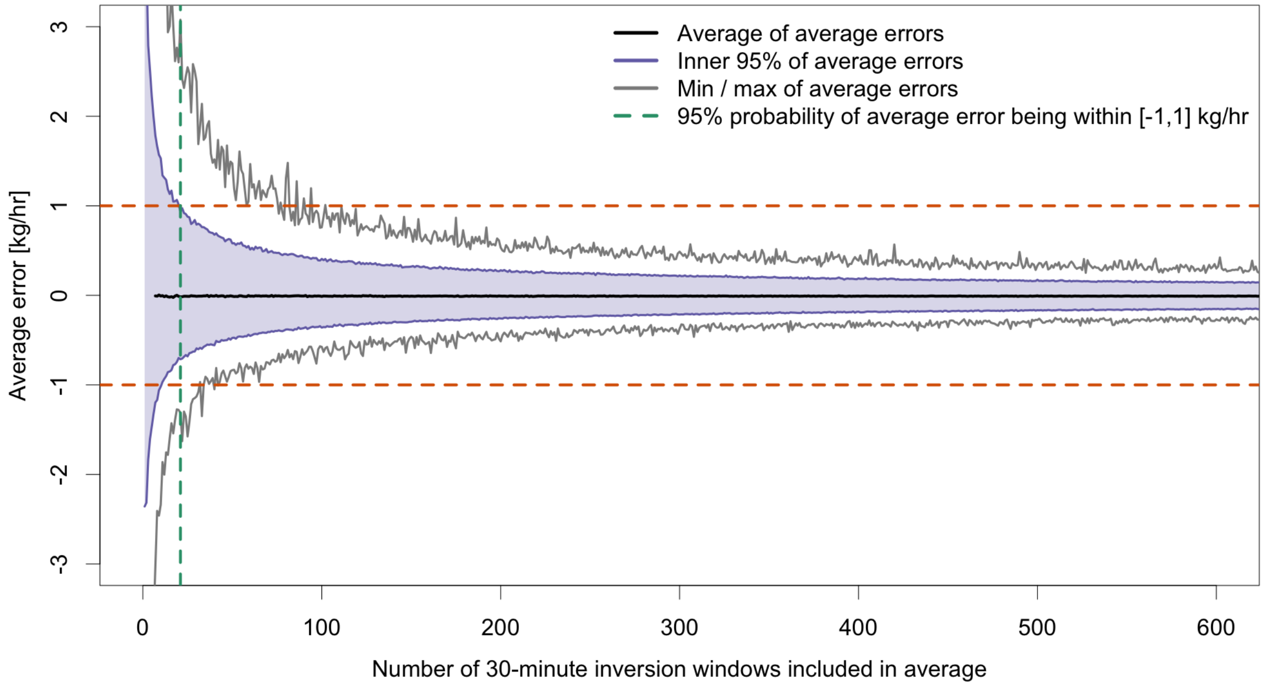


Figure S2: Average error in site-level emission rate estimates from the MDLQ as a function of the number of estimates included in the average. Black line shows the average of the average errors across 5,000 samples. Purple region shows the inner 95% of the average errors. Gray lines show the minimum and maximum of the average errors. Vertical green dashed line shows the point at which the inner 95% of the average errors is bounded by [-1, 1] kg/hr.

## S7 Confusion matrices for source- and site-level detections

Tables 5 through 9 contain source-level confusion matrices based on all available METEC data. These confusion matrices are based on the 30-minute windowed analysis described in Section 3.3 in the main text. That is, the total number of emission state estimates in the following confusion matrices is equal to the number of 30-minute inversion windows in the study period. Estimates of emission state (emitting vs. not emitting) are based on the procedure described in Section 3.4 of the main text.

Table 5: Confusion matrix for the west wellhead.

| | | True Emission State | | |
|---|---|---|---|---|
| | **West Wellhead** | Emission (n = 2,824) | No Emission (n = 8,072) | |
| Predicted Emission State | Emission (n = 3,406) | True Position (TP): 1,910 (17.5%) | False Positive (FP): 1,496 (13.7%) | Positive Predictive Value: $\frac{TP}{TP+FP}$ = 56.1% |
| | No Emission (n = 7,490) | False Negative (FN): 914 (8.4%) | True Negative (TN): 6,576 (60.4%) | Negative Predictive Value: $\frac{TN}{FN+TN}$ = 87.8% |
| | | True Positive Rate: $\frac{TP}{TP+FN}$ = 67.6% | True Negative Rate: $\frac{TN}{FP+TN}$ = 81.5% | Accuracy: $\frac{TP+TN}{TP+FP+FN+TN}$ = 77.9% |

Table 6: Confusion matrix for the west separator.

| | | True Emission State | | |
|---|---|---|---|---|
| | **West Separator** | Emission (n = 3,245) | No Emission (n = 7,699) | |
| Predicted Emission State | Emission (n = 3,281) | True Position (TP): 1,750 (16.0%) | False Positive (FP): 1,531 (14.0%) | Positive Predictive Value: $\frac{TP}{TP+FP}$ = 53.3% |
| | No Emission (n = 7,663) | False Negative (FN): 1,495 (13.7%) | True Negative (TN): 6,168 (56.4%) | Negative Predictive Value: $\frac{TN}{FN+TN}$ = 80.5% |
| | | True Positive Rate: $\frac{TP}{TP+FN}$ = 53.9% | True Negative Rate: $\frac{TN}{FP+TN}$ = 80.1% | Accuracy: $\frac{TP+TN}{TP+FP+FN+TN}$ = 72.4% |

Table 7: Confusion matrix for the tanks.

| | | True Emission State | | |
|---|---|---|---|---|
| | **Tanks** | Emission (n = 3,094) | No Emission (n = 7,682) | |
| Predicted Emission State | Emission (n = 3,961) | True Position (TP): 1,832 (17.0%) | False Positive (FP): 2,129 (19.8%) | Positive Predictive Value: $\frac{TP}{TP+FP}$ = 46.3% |
| | No Emission (n = 6,815) | False Negative (FN): 1,262 (11.7%) | True Negative (TN): 5,553 (51.5%) | Negative Predictive Value: $\frac{TN}{FN+TN}$ = 81.5% |
| | | True Positive Rate: $\frac{TP}{TP+FN}$ = 59.2% | True Negative Rate: $\frac{TN}{FP+TN}$ = 72.3% | Accuracy: $\frac{TP+TN}{TP+FP+FN+TN}$ = 68.5% |

Table 8: Confusion matrix for the east wellhead.

| | | True Emission State | | |
|---|---|---|---|---|
| | **East Wellhead** | Emission (n = 2,936) | No Emission (n = 7,865) | |
| Predicted Emission State | Emission (n =3,134) | True Position (TP): 1,882 (17.4%) | False Positive (FP): 1,252 (11.6%) | Positive Predictive Value: $\frac{TP}{TP+FP}$ = 60.1% |
| | No Emission (n = 7,667) | False Negative (FN): 1,054 (9.8%) | True Negative (TN): 6,613 (61.2%) | Negative Predictive Value: $\frac{TN}{FN+TN}$ = 86.3% |
| | | True Positive Rate: $\frac{TP}{TP+FN}$ = 64.1% | True Negative Rate: $\frac{TN}{FP+TN}$ = 84.1% | Accuracy: $\frac{TP+TN}{TP+FP+FN+TN}$ = 78.7% |

Table 9: Confusion matrix for the east separator.

| | | True Emission State | | |
|---|---|---|---|---|
| | **East Separator** | Emission (n = 3,336) | No Emission (n = 7,258) | |
| Predicted Emission State | Emission (n =3,168) | True Position (TP): 2,024 (19.1%) | False Positive (FP): 1,144 (10.8%) | Positive Predictive Value: $\frac{TP}{TP+FP}$ = 63.9% |
| | No Emission (n = 7,426) | False Negative (FN): 1,312 (12.4%) | True Negative (TN): 6,114 (57.7%) | Negative Predictive Value: $\frac{TN}{FN+TN}$ = 82.3% |
| | | True Positive Rate: $\frac{TP}{TP+FN}$ = 60.7% | True Negative Rate: $\frac{TN}{FP+TN}$ = 84.2% | Accuracy: $\frac{TP+TN}{TP+FP+FN+TN}$ = 76.8% |

Table 10 contains the site-level confusion matrix. The true site-level emission state is determined as follows. If any source is emitting during a given 30-minute inversion window, then the site-level emission state is emitting. If none of the sources are emitting during a given 30-minute window, then the site-level emission state is not emitting. Similarly, if any source is estimated to be emitting (based on the procedure described in Section 3.4 of the main text), then the estimated site-level emission state is emitting. If none of the sources are estimated to be emitting, then the estimated site-level emission state is not emitting.

Table 10: Site-level confusion matrix.

| | | True Emission State | | |
|---|---|---|---|---|
| | **Site-level** | Emission (n = 7,433) | No Emission (n = 4,661) | |
| Predicted Emission State | Emission (n = 7,251) | True Position (TP): 6,147 (50.8%) | False Positive (FP): 1,104 (9.1%) | Positive Predictive Value: $\frac{TP}{TP+FP}$ = 84.8% |
| | No Emission (n = 4,843) | False Negative (FN): 1,286 (10.6%) | True Negative (TN): 3,557 (29.4%) | Negative Predictive Value: $\frac{TN}{FN+TN}$ = 73.4% |
| | | True Positive Rate: $\frac{TP}{TP+FN}$ = 82.7% | True Negative Rate: $\frac{TN}{FP+TN}$ = 76.3% | Accuracy: $\frac{TP+TN}{TP+FP+FN+TN}$ = 80.2% |

# S8 Autocorrelation simulation study

We perform an additional simulation study to verify that the MDLQ model can properly accommodate autocorrelated errors and to evaluate the impact of autocorrelation on a model variant that assumes independent errors. As with the simulation study in Section 4.2 of the main text, we create artificial observations as

$$\tilde{y} = X\beta_T + \tilde{\epsilon},$$

where $\beta_T$ are the true emission rates for each potential source and $\tilde{\epsilon}$ are generated from an AR(1) process. For this study, we test five different AR(1) coefficients: $\{0, 0.25, 0.5, 0.75, 0.95\}$. When then run the MDLQ model as described in Section 3.3 of the main text using $\tilde{y}$ instead of the actual CMS observations. We also run a variant of the MDLQ model on $\tilde{y}$ that assumes independent errors. The left column of Figure S3 shows results using the MDLQ model, and the right column shows results using the variant that assumes independent errors.

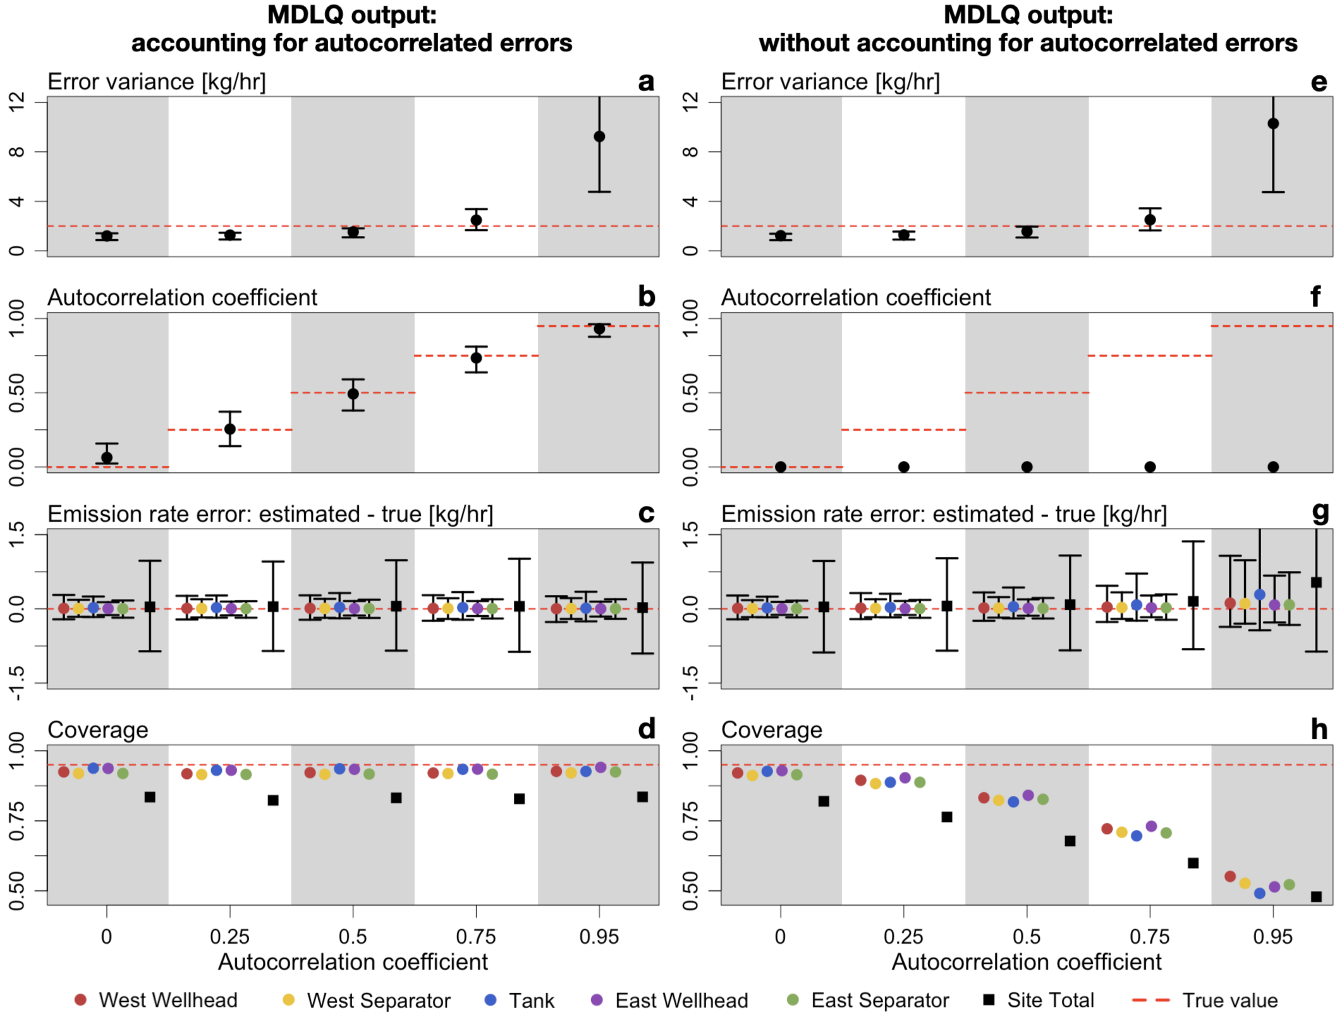


Figure S3: Simulation study varying the degree of autocorrelation in artificial concentration observations. The left column shows results using the MDLQ model described in the main text, and the right column shows results using an MDLQ model variant that assumes independent errors. Red horizontal lines show the true values for each response feature. Bars show the inner 95% range for each value across the inversion windows. Colored circles correspond to source-level results, and black squares correspond to site-level results.

We first consider the MDLQ model results shown in the left column of Figure S3. The MDLQ is able to successfully retrieve the autocorrelation coefficient, $r$, and the emission rate parameters, $\beta$, under different levels of autocorrelation. The coverages of the source-level 95% credible intervals are very close to 95%. As discussed in the main text, the site-level coverage is less than 95% because errors in any of the source-level estimates will propagate to the site-level estimate. Because source-level errors do not always happen at the same time, the site-level 95% credible interval will contain the true emission rate for less than the expected 95% of inversion windows. The inferred error variance, $\sigma^2$, is a function of the correlation coefficient; it is underestimated when there is low autocorrelation and overestimated when there is high autocorrelation. This effect does not bias the inferred emission rate parameters that are of direct interest for source apportionment and will be investigated further in future work.

We now consider the MDLQ model variant that assumes independent errors, with results shown in the right column of Figure S3. We produce these results by fixing the autocorrelation coefficient, $r$, to be identically zero in each iteration of the MCMC. Using this model, emission rates are increasingly overestimated as the amount of autocorrelation increases. Additionally, the coverage of the emission rate parameters decreases as the autocorrelation increases, as this source of variability is not accounted for in the model. Therefore, properly accounting for autocorrelation in the error model is critical for accurate emission rate estimates and credible intervals in the presence of autocorrelated data.

## S9 MDLQ model variant with Laplace errors

We implement a variant of the MDLQ model that assumes a Laplace distribution for the errors. As discussed in Section 4.3 of the main text, we believed that this model would better accommodate large errors from misaligned concentration spikes between the observations and simulation predictions. In this section we fully define this Laplace model variant. As with the MDLQ, we model the concentration observations, $y$, as

$$y = X\beta + \epsilon$$

where the errors are independent and identically distributed according to

$$\epsilon_i \sim \text{Laplace}(0, b)$$

and the scale of the errors, $b$, is given an inverse gamma prior such that

$$b \sim \text{Inv-Gamma}(\alpha_1, \alpha_2).$$

As with the standard MDLQ model, we use a spike-and-slab prior for the $\beta$ parameter. However, given the complicated form of the Laplace likelihood, we are no longer able to integrate out the Dirac delta when deriving the conditional distribution for the spike-and-slab indicator. As such, we use a continuous spike for this model variant, such that the emission rate for each source is modeled as

$$\beta_i \sim \begin{cases} \text{Exp}(p) & z_i = 0 \\ \text{Exp}(s_i) & z_i = 1, \end{cases}$$

where $s >> p$. Specifically, we fix $p = 0.001$ and give each $s_i$ the following prior:

$$s_i \sim \text{Inv-Gamma}(c_i, d_i).$$

We again let the spike-and-slab indicator follow a Bernoulli distribution such that

$$z_i \sim \text{Bernoulli}(\theta_i),$$

where the probability of an emission is given the following prior:

$$\theta_i \sim \text{Beta}(a_i, b_i).$$

Given the complicated form of the Laplace likelihood, we are only able to derive a closed form conditional distribution for $\theta_i$, which takes the same form as the MDLQ model (see Section S3). For the remaining parameters, we update using a Metropolis-Hastings step within the Gibbs sampler. If we again let

$$\xi = \{\beta_1, ..., \beta_p, z_1, ..., z_p, \theta_1, ..., \theta_p, \tau_1^2, ..., \tau_p^2, \sigma^2, \nu, r\},$$

then the remaining update steps are given below. Note that when implemented, we use the log of the following expressions in the Metropolis-Hastings steps. The scale of the Laplace errors, $b$, is given by

$$\begin{aligned}
p(b|\xi) &= p(b|y, \beta) \\
&= p(y|\beta, b)p(b) \\
&\propto \prod_{i=1}^{N} \left( \frac{1}{2b} \exp\left( \frac{-|y_i - X_i^T\beta|}{b} \right) \right) \left(\frac{1}{b}\right)^{\alpha_1+1} \exp\left(\frac{-\alpha_2}{b}\right) \\
&\propto \left(\frac{1}{2b}\right)^{N} \left(\frac{1}{b}\right)^{\alpha_1+1} \exp\left( \sum_{i=1}^{N} \frac{-|y_i - X_i^T\beta|}{b} \right) \exp\left(\frac{-\alpha_2}{b}\right).
\end{aligned}$$

The scale of the slab component of the spike-and-slab prior, $s_i$, is given by

$$\begin{aligned}
p(s_i|\xi) &= p(s_i|\beta_i, z_i) \\
&= p(\beta_i|s_i, z_i)p(s_i) \\
&\propto \begin{cases} (1-z_i)\left(\frac{1}{p}\right)\exp\left(\frac{\beta_i}{p}\right) + (z_i)\left(\frac{1}{s_i}\right)\exp\left(\frac{\beta_i}{s_i}\right)\left(\frac{1}{s_i}\right)^{c_i+1}\exp\left(\frac{-d_i}{s_i}\right), & \beta_i \geq 0 \\ 0, & \beta_i < 0, \end{cases}.
\end{aligned}$$

The emission rates for each source, $\beta_i$, is given by

$$\begin{aligned}
p(\beta_i|\xi) &= p(\beta_i|y, \beta_{-i}, b, z_i, s_i) \\
&\propto p(y|\beta, b)p(\beta_i|z_i, s_i) \\
&\propto \prod_{i=1}^{N} \left( \frac{1}{2b} \exp\left( \frac{-|y_i - X_i^T\beta|}{b} \right) \right) \left\{ (1-z_i)\left(\frac{1}{p}\right)\exp\left(\frac{-\beta_i}{p}\right) + (z_i)\left(\frac{1}{s_i}\right)\exp\left(\frac{-\beta_i}{s_i}\right) \right\} \\
&\propto \left(\frac{1}{2b}\right)^{N} \exp\left( \sum_{i=1}^{N} \frac{-|y_i - X_i^T\beta|}{b} \right) \left\{ (1-z_i)\left(\frac{1}{p}\right)\exp\left(\frac{-\beta_i}{p}\right) + (z_i)\left(\frac{1}{s_i}\right)\exp\left(\frac{-\beta_i}{s_i}\right) \right\}.
\end{aligned}$$

As with the MDLQ model, the spike-and-slab indicator, $z_i$, can be written as

$$p(z_i|\xi) = \text{Bernoulli}(\psi_i),$$

where

$$\psi_i = \frac{p(z_i = 1|\xi)}{p(z_i = 0|\xi) + p(z_i = 1|\xi)}.$$

We now consider the $z_i = 1$ and $z_i = 0$ cases separately. First, consider $z_i = 1$. We get that

$$\begin{aligned} p(z_i = 1|\xi) &= p(z_i = 1|\beta_i, s_i, \theta_i) \\ &\propto p(\beta_i|z_i = 1, s_i, \theta_i)p(z_i = 1|\theta_i) \\ &\propto \left(\frac{1}{s_i}\right)\exp\left(\frac{-\beta_i}{s_i}\right)\theta_i. \end{aligned}$$

Now consider $z_i = 0$. We get that

$$\begin{aligned} p(z_i = 0|\xi) &= p(z_i = 0|\beta_i, s_i, \theta_i) \\ &\propto p(\beta_i|z_i = 0, s_i, \theta_i)p(z_i = 1|\theta_i) \\ &\propto \left(\frac{1}{p}\right)\exp\left(\frac{-\beta_i}{p}\right)(1-\theta_i). \end{aligned}$$

This gives us the following expression for the conditional distribution for $z_i$:

$$\psi_i = \frac{\left(\frac{1}{s_i}\right)\exp\left(\frac{-\beta_i}{s_i}\right)\theta_i}{\left(\frac{1}{p}\right)\exp\left(\frac{-\beta_i}{p}\right)(1-\theta_i) + \left(\frac{1}{s_i}\right)\exp\left(\frac{-\beta_i}{s_i}\right)\theta_i},$$

where again

$$p(z_i|\xi) = \text{Bernoulli}(\psi_i).$$

# S10 Form of the correlation matrix: R

As discussed in Section 3.1.1 of the main text, the data layer of the MDLQ model takes the form

$$\boldsymbol{y} = X\boldsymbol{\beta} + \boldsymbol{\epsilon},$$

where the errors $\boldsymbol{\epsilon} \equiv \{\epsilon_1, ..., \epsilon_n\}$ follow a multivariate normal, such that $\boldsymbol{\epsilon} \sim N(0, \sigma^2 R)$. We assume that $\boldsymbol{\epsilon}$ follow an AR(1) autocorrelation model, and as such, the R matrix takes the following form:

$$R = \begin{bmatrix} 1 & r & r^2 & \dots & r^{n-1} \\ r & 1 & r & \dots & \vdots \\ r^2 & r & 1 & \dots & \vdots \\ \vdots & \vdots & \vdots & \ddots & \vdots \\ r^{n-1} & \dots & \dots & \dots & 1 \end{bmatrix}.$$

## S11 Methane concentration data example from all sensors

Figure S4 shows the methane concentration measurements from all 10 CMS sensors on the METEC site during the example time period shown in Figure 2 in the main manuscript.

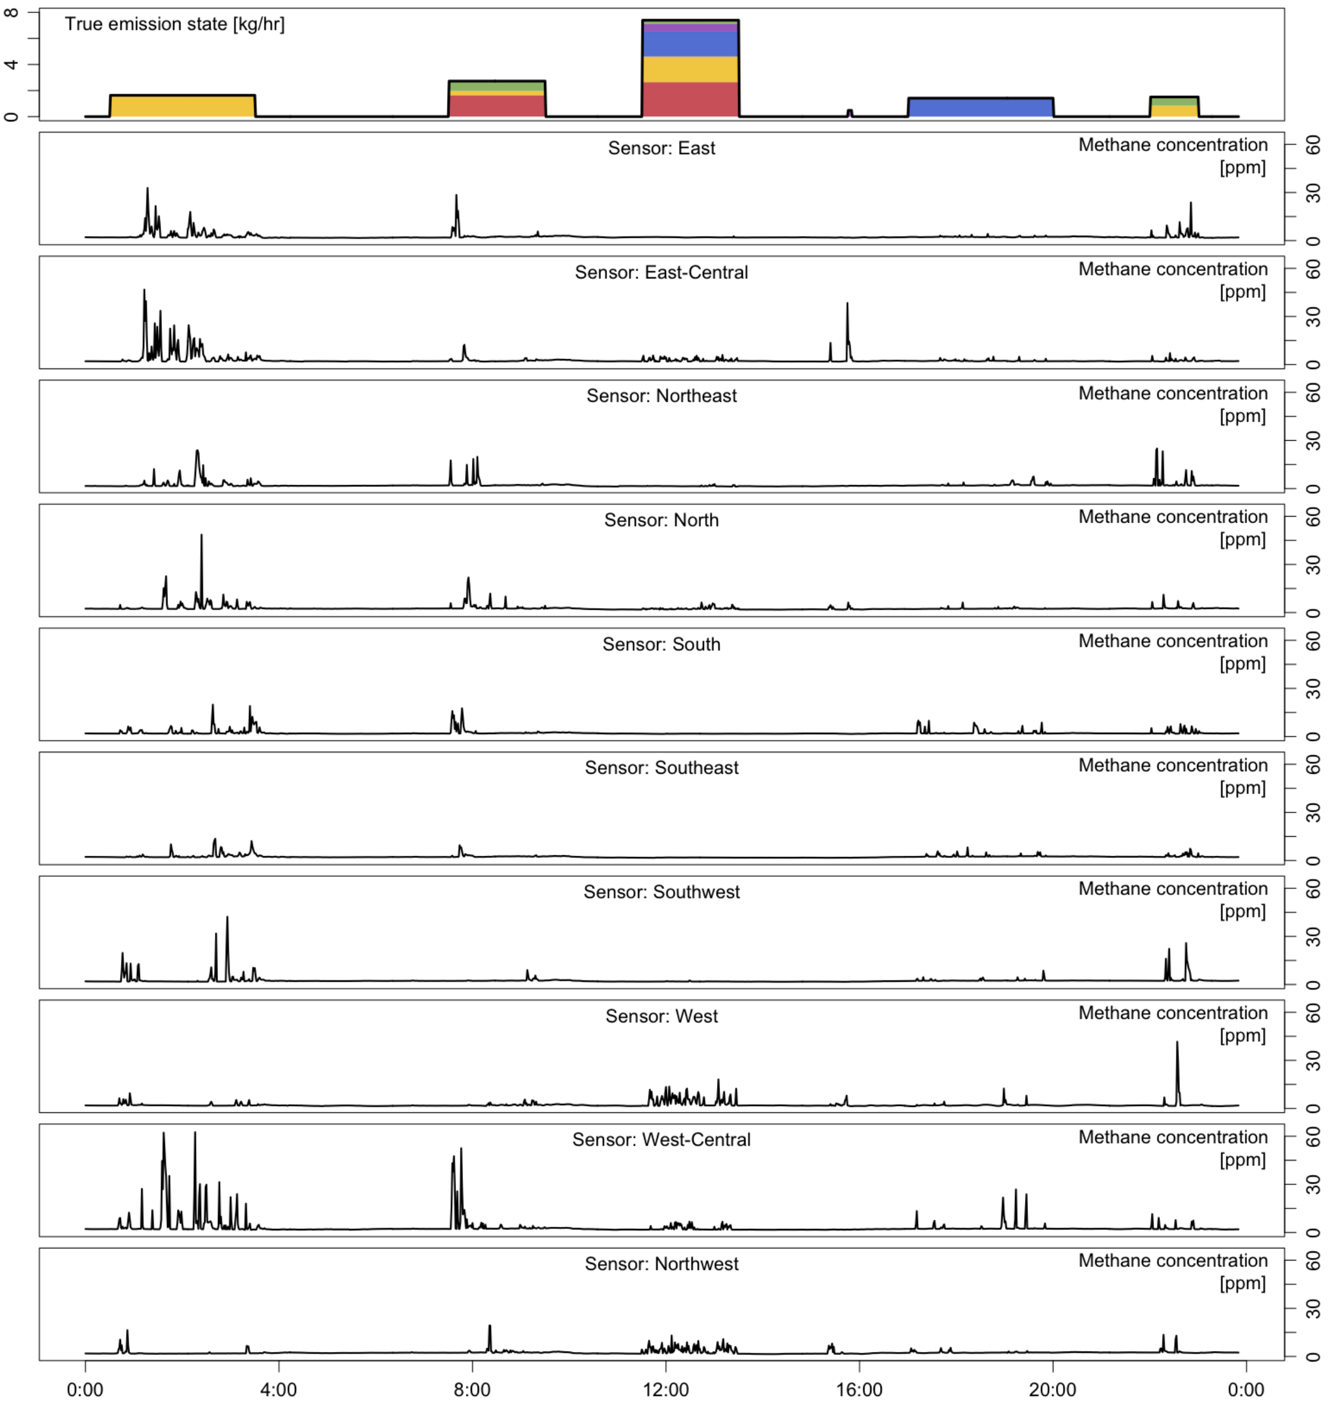


Figure S4: *Example data from February 12, 2024. Top plot shows the true emission state, and all remaining plots show the methane measurements from the 10 CMS sensors on the METEC site.*

## References


[1] R.M. Young Company, "ResponseONE Ultrasonic Anemometer Model 91000," Tech. Rep. 91000-90(F), 2021. https://www.youngusa.com/wp-content/uploads/2016/12/91000-90F.pdf.

[2] F. Pasquill, "The estimation of the dispersion of windborne material," *Meteorological Magazine*, vol. 90, pp. 33–49, 1961.

[3] B. D. Turner, "Workbook of atmospheric dispersion estimates," Tech. Rep. 742-R-70-001, U.S. Environmental Protection Agency, 1970.

[4] EPA, "Workbook for plume visual impact screening and analysis (revised)," Tech. Rep. 450-4-88-015, U.S. Environmental Protection Agency, 1992.

[5] F. Dablander, "Variable selection using Gibbs sampling," Mar. 2019. https://fabiandablander.com/r/Spike-and-Slab.html.

[6] C. G. Small, *Expansions and Asymptotics for Statistics*. New York: Chapman and Hall/CRC, May 2010.
